# Supplementary material for: V3GAN: Decomposing Background, Foreground and Motion for Video Generation
Source: arXiv:2203.14074 source file (2022-03-26)

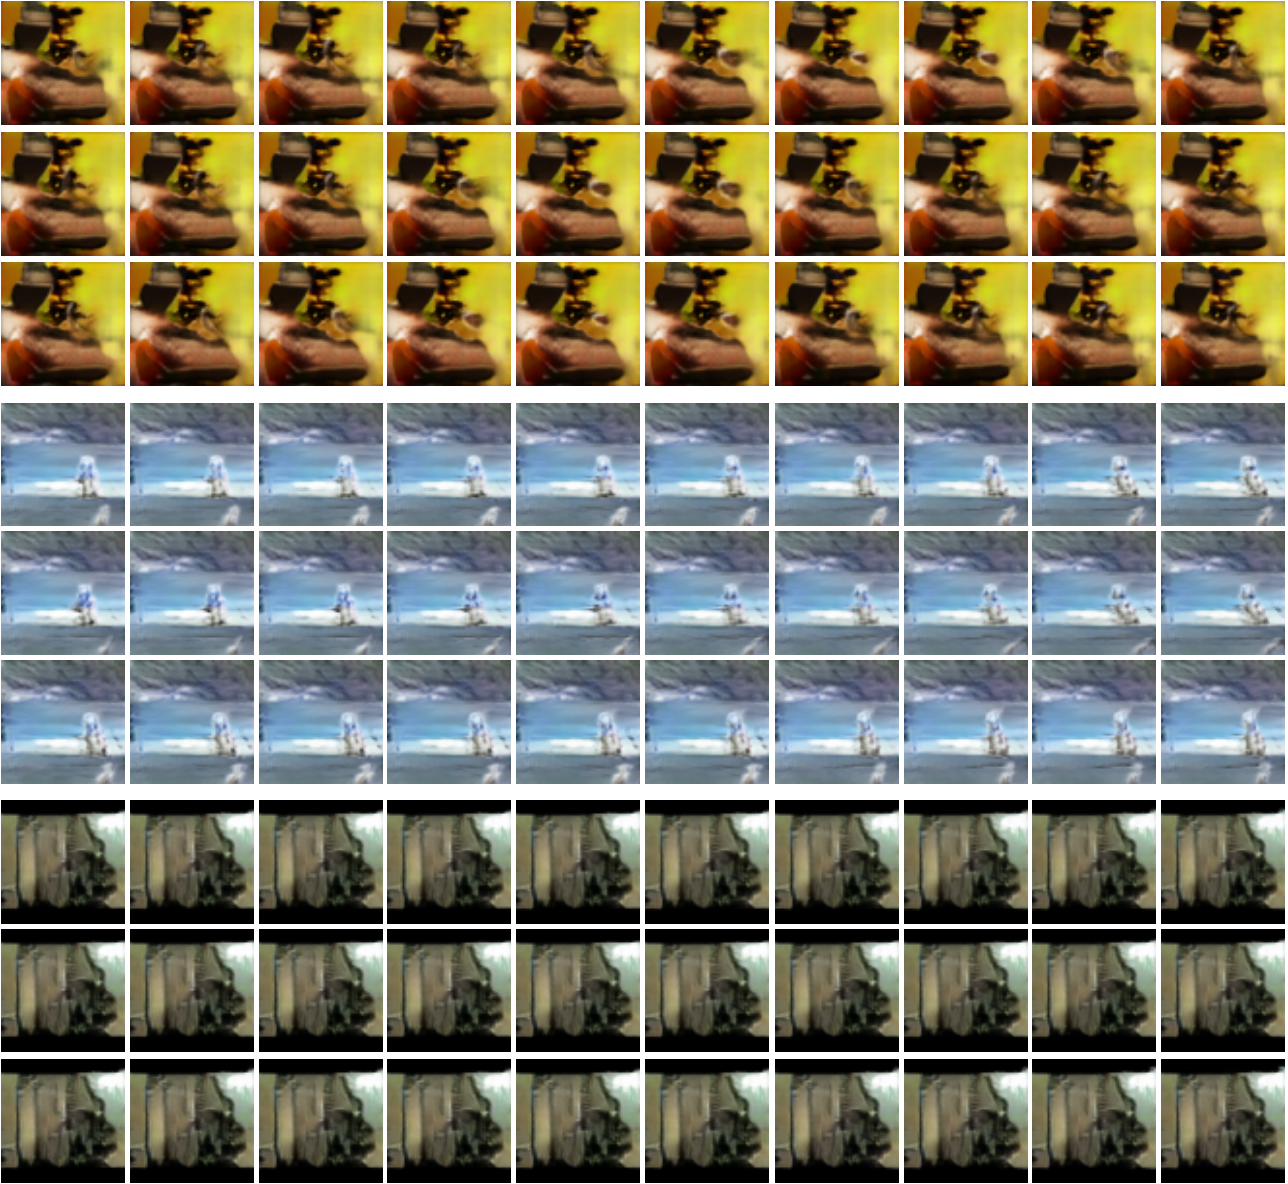

Supplement: Supplementary file 1 [file UCF-qual-noise-ablation.pdf]
